# Supplementary material for: LM Agents for Coordinating Multi-User Information Gathering
Source: arXiv:2502.12328 source file (2025-02-17)
Supplement: Supplementary file 1 [file cinema.tex]

Alice Anastasiou-to-Bot [login]: [LOGIN]
Alice Anastasiou-to-Bot [chat]:  What are all the locations with a cinema? 
	>>>  Reflection.thought("I will first resolve the primary user to get the right contact information")
	>>>  Enterprise.resolve_primary_user()
{"email": "alice@contoso.com", "full_name": "Alice Anastasiou", "user_id": "alice@contoso.com"}
	>>>  Reflection.thought("I will search user documents to see if the user request can be answered directly")
	>>>  EnterpriseSearch.search_documents(query="locations with a cinema")
('Document(url=\'cinema/film\', title=\'film\', content=\'[{"film id": 1, "rank in series": 26, "number in season": 1, "title": "The Case of the Mystery Weekend", "directed by": "Bill Schreiner", "original air date": "September 21\\\\u201325, 1992", "production code": "50021\\\\u201350025"}, {"film id": 2, "rank in series": 27, "number in season": 2, "title": "The Case of the Smart Dummy", "directed by": "Bill Schreiner", "original air date": "September 28\\\\u2013October 2, 1992", "production code": "50231\\\\u201350235"}, {"film id": 3, "rank in series": 28, "number in season": 3, "title": "The Case: Off the Record", "directed by": "Bill Schreiner", "original air date": "October 5\\\\u20139, 1992", "production code": "50011\\\\u201350015"}, {"film id": 4, "rank in series": 29, "number in season": 4, "title": "The Case of the Bermuda Triangle", "directed by": "Jesus Salvador Trevi\\\\u00f1o", "original air date": "October 12\\\\u201316, 1992", "production code": "50251\\\\u201350255"}, {"film id": 5, "rank in series": 30, "number in season": 5, "title": "The Case of the Piggy Banker", "directed by": "Bill Schreiner", "original air date": "October 19\\\\u201323, 1992", "production code": "50241\\\\u201350245"}]\')',)
	>>>  Reflection.thought("User documents do not have information about locations with a cinema. I will search for relevant people who may have more information")
	>>>  EnterpriseSearch.search_relevant_people(query="locations with a cinema")
{"sylvie": " The user might have information about cinemas, including their names, opening years, capacities, and locations.", "harpreet": " The user might have information about cinemas, including their names, opening years, capacities, and locations.", "bhushan": " The user might have information about cinema schedules, including the cinema id, film id, date, show times per day, and price."}
	>>>  Reflection.thought("I can reach out to Sylvie, Harpreet, and Bhushan who seem to have more information about cinemas. I will confirm with Alice if that is okay")
	>>>  Enterprise.send_message("alice@contoso.com", "Hi Alice, I couldn't find enough information in your documents to compile that directly. I can reach out to Sylvie, Harpreet, and Bhushan who may have more information about cinemas and their locations. Sounds good?")
	>>>  System.finish()
Bot-to-Alice Anastasiou [chat]: Hello, I'm here to help you as your M365 Copilot!
Bot-to-Alice Anastasiou [chat]: Hi Alice, I couldn't find enough information in your documents to compile that directly. I can reach out to Sylvie, Harpreet, and Bhushan who may have more information about cinemas and their locations. Sounds good?
Alice Anastasiou-to-Bot [chat]:  Yes, please do. 
	>>>  Reflection.thought("Alice has confirmed that I can reach out to Sylvie, Harpreet, and Bhushan. I will start by reaching out to Sylvie for the locations with a cinema")
	>>>  Enterprise.resolve_person("Sylvie")
{"email": "sylvie@contoso.com", "full_name": "Sylvie Rocher", "user_id": "sylvie"}
	>>>  Enterprise.send_message("sylvie@contoso.com", "Hi Sylvie, Can you please tell me all the locations with a cinema?", title="Information needed about cinemas")
	>>>  System.finish()
Bot-to-Alice Anastasiou [secondary_user_join]: [A NEW CHALLENGER APPROACHES]
Bot-to-Sylvie Rocher [chat]: Hi Sylvie, Can you please tell me all the locations with a cinema?
Sylvie Rocher-to-Bot [chat]:  The locations with a cinema are County Wicklow, County Cork, County Dublin, County Clare, and County Tipperary. 
	>>>  Reflection.thought("Sylvie has provided the information about locations with a cinema. I will send this information to Alice")
	>>>  Enterprise.send_message("alice@contoso.com", "Hi Alice, the locations with a cinema are: - County Wicklow - County Cork - County Dublin - County Clare - County Tipperary Let me know if you need more information!", title="Locations with a cinema")
	>>>  System.finish()
Bot-to-Alice Anastasiou [chat]: Hi Alice, the locations with a cinema are: - County Wicklow - County Cork - County Dublin - County Clare - County Tipperary Let me know if you need more information!
Alice Anastasiou-to-Bot [chat]:   No, that's all I needed. Thank you! 
	>>>  Reflection.thought("Alice has confirmed that no more information is needed. I will close the session")
	>>>  Enterprise.send_session_completed()
	>>>  System.finish()
Bot-to-Alice Anastasiou [session_completed]: Session completed.
