# Supplementary material for: LM Agents for Coordinating Multi-User Information Gathering
Source: arXiv:2502.12328 source file (2025-02-17)
Supplement: Supplementary file 2 [file party-people.tex]

% \begin{lstlisting}[breaklines=true, caption={An example trace, with \reactagent{} when using GPT-4-turbo as LLM.}, label={ls:qualparty}]

% # Alice Anastasiou says: Return the names of parties that have two or more events. 
% >>>  Reflection.thought("I will first resolve the primary user to get the right contact information")
% >>>  Enterprise.resolve_primary_user()
% {"email": "alice@company.com", "full_name": "Alice Anastasiou", "user_id": "alice@company.com"}
% >>>  Reflection.thought("I will search user documents to see if the user request can be answered directly")
% >>>  EnterpriseSearch.search_documents("parties with two or more events")
% ('Document(url=\'party_people/region\', title=\'region\', content=\'[{"region id": 1, "region name": "United Kingdom", "date": "1 July 2002", "label": "Parlophone", "format": "CD", "catalogue": "540 3622"}, {"region id": 2, "region name": "United Kingdom", "date": "1 July 2002", "label": "Parlophone", "format": "2\\\\u00d7 LP", "catalogue": "539 9821"}, {"region id": 3, "region name": "Japan", "date": "3 July 2002", "label": "Toshiba-EMI", "format": "CD", "catalogue": "TOCP-66045"}, {"region id": 4, "region name": "United States", "date": "16 July 2002", "label": "Astralwerks", "format": "CD", "catalogue": "ASW 40362"}, {"region id": 5, "region name": "United States", "date": "16 July 2002", "label": "Astralwerks", "format": "CD digipak", "catalogue": "ASW 40522"}]\')',)
% >>>  Reflection.thought("The document does not contain information about parties and their events. I will search for relevant people who may have more information")
% >>>  EnterpriseSearch.search_relevant_people("parties with two or more events")
% {"gorosti": " The user might have information about parties, including the party name, minister, office tenure, and region.", "cassie": " The user might have information about political parties, including the party name, minister, office tenure, and region.", "bhushan": " The user might have information about members, including their names, party affiliations, and office status."}
% >>>  Reflection.thought("I can reach out to Gorosti, Cassie, and Bhushan who seem to have more information about parties. I will confirm with Alice if that is okay")
% >>>  Enterprise.send_message("alice@company.com", "Hi Alice, I couldn't find enough information in your documents to compile that directly. I can reach out to Gorosti, Cassie, and Bhushan who may have more information. Sounds good?")
% >>>  System.finish()

% # Alice Anastasiou says:  Yes, please reach out to them. 
% >>>  Reflection.thought("Alice has confirmed that I can reach out to Gorosti, Cassie, and Bhushan. I will start by reaching out to Gorosti for the names of parties that have two or more events")
% >>>  Enterprise.resolve_person("Gorosti")
% {"email": "gorosti@company.com", "full_name": "Gorosti Egiagarai", "user_id": "gorosti"}
% >>>  Enterprise.send_message("gorosti@company.com", "Hi Gorosti, Can you please tell me the names of parties that have two or more events?", title="Information needed about parties")
% >>>  System.finish()

% # Gorosti Egiagarai says:  I do not have information on the number of events for each party. 
% >>>  Reflection.thought("Gorosti does not have information on the number of events for each party. I will reach out to Cassie for the same information")
% >>>  Enterprise.resolve_person("Cassie")
% {"email": "cassie@company.com", "full_name": "Cassie Hicks", "user_id": "cassie"}
% >>>  Enterprise.send_message("cassie@company.com", "Hi Cassie, Can you please tell me the names of parties that have two or more events?", title="Information needed about parties")
% >>>  System.finish()

% # Cassie Hicks says:  I do not have information on the number of events for each party. 
% >>>  Reflection.thought("Cassie also does not have information on the number of events for each party. I will reach out to Bhushan for the same information")
% >>>  Enterprise.resolve_person("Bhushan")
% {"email": "bhushan@company.com", "full_name": "Bhushan Magar", "user_id": "bhushan"}
% >>>  Enterprise.send_message("bhushan@company.com", "Hi Bhushan, Can you please tell me the names of parties that have two or more events?", title="Information needed about parties")
% >>>  System.finish()

% # Bhushan Magar says:  Sorry, I do not have that information. 
% >>>  Reflection.thought("Bhushan also does not have the requested information. I will inform Alice that I could not find the information she requested.")
% >>>  Enterprise.send_message("alice@company.com", "Hi Alice, I reached out to Gorosti, Cassie, and Bhushan, but unfortunately, none of them had the information on the names of parties that have two or more events. I'm sorry I couldn't fulfill your request this time. Let me know if there's anything else I can assist you with!", title="Information about parties")
% >>>  System.finish()

% # Alice Anastasiou says:   That's okay, thank you for trying. 
% >>>  Reflection.thought("Alice has acknowledged the effort and does not require further assistance. I will close the session")
% >>>  Enterprise.send_session_completed()
% >>>  System.finish()  # Closing the session as per the user's acknowledgment and no further assistance required.
% \end{lstlisting}
